# Supplementary material for: Less is More: Focus Attention for Efficient DETR
Source: arXiv:2307.12612 source file (2023-07-24)
Supplement: Supplementary file 1 [file supp.pdf]

# Less is More: Focus Attention for Efficient DETR

Anonymous ICCV submission

Paper ID 5415

## Abstract

DETR-like models have significantly boosted the performance of object detectors and even outperformed classical convolution-based models. However, all tokens are treated equally without discrimination also brings a redundant computational burden of detectors and *limit information interaction between queries in the encoder*. *especially for the encoder*. The recent sparsification strategies exploit a subset of informative tokens to reduce attention complexity in the encoder while maintaining the model performance. *However, they only apply to specific model structures and still fail to interact between queries. In this paper* To address these issues, we propose Focus-DETR, which focuses attention on more informative tokens for a better trade-off between computation efficiency and model accuracy. Specifically, we design a token scoring mechanism that considers both localization and category semantic information of the object from multi-scale feature maps, *which is beneficial to efficiently abandon the background queries and enhance the semantic interaction of the fine-grained object queries through the pyramid encoder. together with an enhanced self-attention module concerning these tokens to boost the final detection results.* Compared with the state-of-the-art sparse transformed-based detector under the same setting, our Focus-DETR gets comparable complexity while achieving 50.4AP (+2.2) on COCO. The code will be available upon acceptance.

## 1. Introduction

Object detection is a fundamental task in computer vision that aims to predict the bounding boxes and classes of objects in an image, as shown in Fig. 1 (a), which is of great importance in real-world applications. ~~such as smart cities, autonomous driving, industrial robot, image retrieval, etc.~~ DETR proposed by Carion *et al.* [1] uses learnable queries to probe image features from the output of Transformer encoders and bipartite graph matching to perform set-based box prediction. DETR-like models [18, 35, 14, 32, 21, 25, 2, 30, 36] have made remarkable

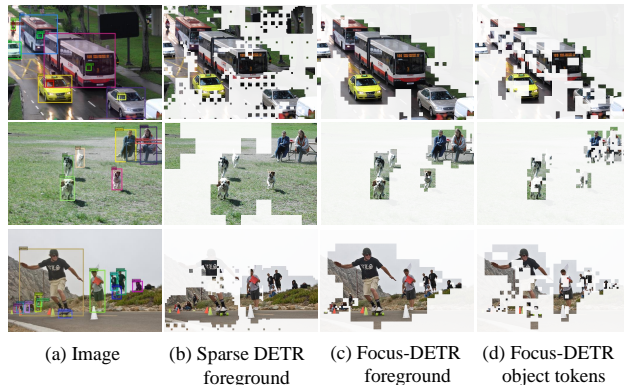

Figure 1: Visualization and comparison of tokens selected by Sparse DETR [25] and our Focus-DETR. (a) is the original images, (b) and (c) represent the foreground selected by models. (d) indicates the object tokens for the Object Enhanced Self-attention Module (OESM). Patches with smaller sizes come from higher-level features.

progress and gradually bridged the gap with the detectors based on convolutional neural networks.

Global attention in the DETR-like models improves the detection performance but suffers from computational burden and inefficiency due to redundant calculation without explicit discrimination for all tokens. To tackle this issue, Deformable DETR [36] reduces the quadratic complexity to linear complexity through key sparsification, and it has developed into a mainstream paradigm due to the advantages of leveraging multi-scale features. Herein, we further analyze the computational burden *and latency* of components in these models (Fig. 2). As shown in Fig. 2, we observe that the calculation cost of the encoder is  $8.8\times$  that of the decoder in Deformable DETR [36] and  $7.0\times$  in DINO [35]. *In addition, the latency of the encoder is approximately 4~8 times that of the decoder in Deformable DETR and DINO,* which emphasizes the necessity to improve the efficiency in the encoder module. In line with this, previous works have generally discussed the feasibility of compressing tokens in the transformer encoder. For instance, PnP-DETR [29] abstracts the whole features into fine fore-

ground object feature vectors and a small number of coarse background contextual feature vectors. In a recent study, Sparse DETR [25] proposes to preserve the 2D spatial structure of the tokens through query sparsity, which makes it applicable to Deformable DETR [36] to utilize multi-scale features. By leveraging the cross-attention map in the decoder as the token importance score, Sparse DETR achieves performance comparable to Deformable DETR only using 30% of queries in the encoder.

Despite all the progress, the current models [29, 25] are still challenged by sub-optimal token selection strategy. As shown in Fig. 1 (b), the selected tokens contain a lot of noise and some important object tokens are obviously overlooked. In particular, Sparse DETR’s supervision of the foreground predictor relies heavily on the decoder’s cross-attention map (DAM), which may introduce noise in the training process. **Preliminary experiments show severe performance decay when the Sparse DETR is embedded into the models using learnable queries. In this case, foreground selection will be misled due to the weak correlation between DAM and the sparse foreground queries. Furthermore, Sparse DETR is insufficient to make full use of multi-scale feature maps. Moreover, this unsophisticated foreground selection is challenging to focus on more fine-grained features critical to boosting detection performance. Moreover, the number of retained foreground tokens remains numerous, and performing the query interaction without more fine-grained selection is not feasible due to computational cost limitations.**

To address these issues, we propose Focus-DETR to allocate attention to more informative tokens by stacking the localization information and category semantic information. **Firstly, we design a scoring mechanism to determine the semantic level of tokens. we design a Foreground Token Selector (FTS) aims to abandon background tokens based on top-down score modulations across multi-scale features. We assign positive and negative labels to all tokens from the backbone with reference to the ground truth and predict the foreground probability. The score of the higher-level tokens from multi-scale feature maps modulates the lower-level ones to impose the validity of selection further. To introduce semantic information into the token selection process, we design a multi-category score predictor. The foreground and category scores will jointly determine the more fine-grained tokens with strong category semantics, as shown in Fig. 1 (d). to select more fine-grained tokens. Then, the selected tokens interact with each other through the Object Enhanced Self-attention Module (OESM) embedded in the encoder to remedy limitation of deformable attention in distant information mixing. And then, we reconstruct a calculation prototype termed Pyramid Encoder to process tokens with different semantic levels. Thus, the limitation of deformable attention in distant information mixing is remedied, and then the semantic information of foreground**

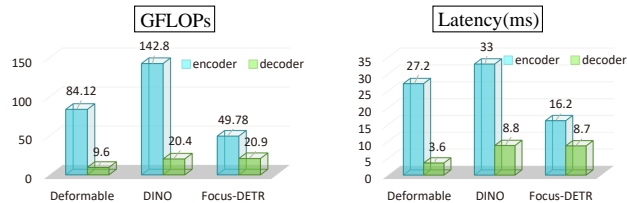

Figure 2: Distribution of calculation cost and latency in the Transformer part of the DETR-like models, e.g., Deformable DETR [36], DINO [35] and our Focus-DETR.

**queries is enhanced by fine-grained token updates.**

To sum up, Focus-DETR obtains more accurate foreground information and focuses on fine-grained tokens by gradually introducing semantic information, and further enhances fine-grained tokens with minimal computational cost. Extensive experiments validate the performance of the proposed method for focusing attention on necessary tokens. **Furthermore, Focus-DETR is general for DETR-like models that use different query construction strategies.** For example, our method can achieve 50.4AP (+2.2) on COCO compared to Sparse DETR with a similar computation cost under the same setting.

## 2. Related work

**Transformer-based detectors.** Recently, Carion *et al.*[1] proposed an end-to-end object detector named DETR (DEtection TRansformer) based on Vision Transformer [7] architecture. DETR transforms object detection into a set prediction task through the backbone, encoder, and decoder and supervises the training process through Hungarian matching algorithms. A lot of recent works[18, 14, 36, 35, 21, 3, 34, 2, 4] have boosted the performance of Transformer-based detectors from the perspective of accelerating training convergence and improving detection precision. Representatively DINO[35] establishes DETR-like models as a mainstream detection framework, not only for its novel end-to-end detection optimization, but also for its superior performance. Fang *et al.* [8] propose YOLOS and reveal that object detection can be accomplished in a pure sequence-to-sequence manner with minimal additional inductive biases. Li *et al.*[15] propose ViTDet to explore the plain, non-hierarchical ViT as a backbone network for object detection. Dai *et al.*[5] propose a pretext task named random query patch detection to Unsupervisedly Pre-train DETR (UP-DETR) for object detection. IA-RED<sup>2</sup> [22] introduces an interpretable module for dynamically discarding redundant patches.

**Lightweight Vision Transformers.** As we all know, vision Transformer (ViT) suffers from its high calculation

complexity and memory cost. Lu *et al.* [23] propose an efficient ViT with dynamic sparse tokens to accelerate the inference process. Yin *et al.* [33] adaptively adjust the inference cost of ViT according to the complexity of different input images. Xu *et al.* [31] propose a structure-preserving token selection strategy and a dual-stream token update strategy to significantly improve model performance without changing the network structure. Tang *et al.* [27] presents a top-down layer by layer patch slimming algorithm to reduce the computational cost in pre-trained Vision Transformers. The core strategy of these algorithms and other similar works [11, 13, 19] is to abandon redundant tokens to reduce the computational complexity of the model.

In addition to the above models focused on sparsity backbone structure applied on classification tasks, some works [25, 29] lie in reducing the redundant calculation in DETR-like models. Efficient DETR [32] reduces the number of layers of the encoder and decoder by optimizing the structure while keeping the performance unchanged. PnP-DETR and Sparse DETR have achieved performance comparable to DETR or Deformable by abandoning background tokens with weak semantics. However, these methods are suboptimal in judging background information and lack enhanced attention to more fine-grained features.

### 3. Methodology

In this section, we first describe the overall architecture of the proposed Focus-DETR. Then, we elaborate our core contributions: (a) constructing a scoring mechanism that considers both localization and **category** semantic information from multi-scale feature maps. **Thus we obtain two-level explicit discrimination for foreground and fine-grained object tokens.**; (b) **proposing an enhanced lightweight self-attention module using more salient tokens to boost the final detection results. Based on the reliable scoring mechanism, we reconstruct a calculation prototype termed Pyramid Encoder to process tokens with different semantic levels, which balances model performance, resource consumption, and response latency.** A detailed analysis of the computational complexity of the deformable attention and our proposed components is also provided.

#### 3.1. Model Architecture

As shown in Fig. 3, ~~similar to other DETR-like models,~~ Focus-DETR is composed of a backbone network, a Transformer encoder, and a Transformer decoder. The backbone can be equipped with ResNet [10] or Swin Transformer [20]. To leverage multi-scale features  $\{\mathbf{f}_l\}_{l=1}^L$  ( $L = 4$ ) from the backbone, where  $\mathbf{f}_l \in \mathbb{R}^{C \times H_l \times W_l}$ , we obtain the feature maps  $\{\mathbf{f}_1, \mathbf{f}_2, \mathbf{f}_3\}$  in three different scales (*i.e.*, 1/8, 1/16, 1/32) and downsample  $\mathbf{f}_3$  to get  $\mathbf{f}_4$  (*i.e.*, 1/64).

Before being fed into the Transformer encoder, the multi-scale feature maps  $\{\mathbf{f}_l\}_{l=1}^L$  first go through a fore-

ground token selector (Section 3.2) which uses a series of top-down score modulations to indicate whether a token belongs to the foreground. Then, the selected foreground tokens of each layer will pass through a multi-category score predictor to select tokens with higher objectiveness score by leveraging foreground information and semantic information (Section 3.2). These object tokens will interact further with each other **and complement the semantic limitation of the foreground queries through the proposed Pyramid Encoder.** ~~through the proposed Object Enhanced Self-attention Module (Section 3.3) before the conventional deformable attention layers.~~

#### 3.2. Foreground Token Selector **Scoring mechanism**

**Foreground Token Selector.** Sparse DETR [25] has demonstrated that only involving a subset of tokens for encoders can achieve comparable detection performance. However, as illustrated in Fig. 4, the token selection provided by Sparse DETR [25] has many drawbacks. In particular, we notice that many preserved tokens do not align with foreground objects.

~~As discussed earlier,~~ **We think** the challenge faced by Sparse DETR lies in that its supervision of token selection relies heavily on the attention map from the decoder **DAM.** ~~As the attention map is also generated by the model,~~ **The correlation between DAM and retained foreground tokens will be reduced when using learnable queries, which may bring errors during training. introduce noise in training process.** Therefore, instead of predicting this kind of pseudo-ground truth [25], we leverages ground truth boxes and labels to supervise the foreground token selection inspired by [17]. To properly provide a binary label for each token on whether it appears in the foreground, we design a label assignment protocol to leverage the multi-scale feature maps for objects with different scales.

In particular, ~~we first set a range of sizes for the bounding boxes of different feature maps. Different from the traditional approaches [28] for multi-scale feature label assignment we first set a range of sizes and add the overlap of the adjacent interval by 50% to enhance the prediction near on the boundary.~~ Formally, for each token  $t_l^{(i,j)}$  with stride  $s_l$ , where  $l$  is the index of scale level, and  $(i, j)$  is the position in the feature map, we denote the corresponding coordinate  $(x, y)$  in the original image as  $(\lfloor \frac{s_l}{2} \rfloor + i \cdot s_l, \lfloor \frac{s_l}{2} \rfloor + j \cdot s_l)$ . Considering the adjacent feature map, our protocol determines the label  $l_l^{(i,j)}$  according to the following rules, *i.e.*,

$$l_l^{(i,j)} = \begin{cases} 1, & (x, y) \in \mathcal{D}_{Bbox} \wedge d_l^{(i,j)} \in [r_b^l, r_e^l] \\ 0, & (x, y) \notin \mathcal{D}_{Bbox} \vee d_l^{(i,j)} \notin [r_b^l, r_e^l] \end{cases}, \quad (1)$$

where  $d_l^{(i,j)}$  represents the maximum checkerboard distance between  $(x, y)$  with the center of the bounding box,  $\mathcal{D}_{Bbox}$



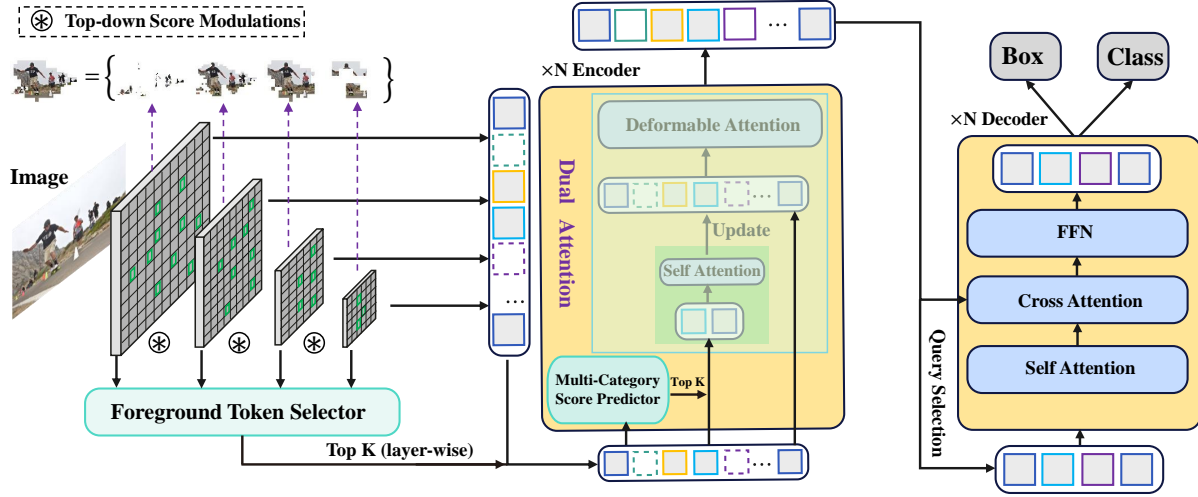

Figure 3: The architecture overview of the proposed Focus-DETR. Our Focus-DETR comprises a backbone network, a Transformer encoder, and a Transformer decoder. We design a foreground token selector (FTS) based on top-down score modulations across multi-scale features. And the selected tokens by a multi-category score predictor go through the Object Enhanced Self-attention Module (OESM) to remedy the limitation of deformable attention in distant information mixing.

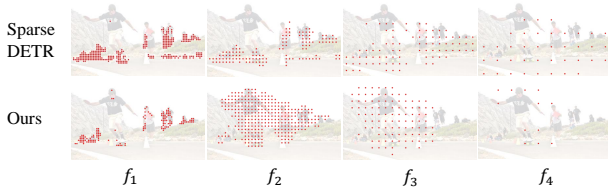

Figure 4: The foreground tokens preserved in different feature maps of Sparse DETR and our Focus-DETR. The red dots indicate the position of the reserved token corresponding to the original image based on the stride.

denotes the ground truth label of bounding boxes,  $[r_b^l, r_e^l]$  represents the maximum and minimum value of object predicted by the  $l$ -layer feature map and  $r_b^l < r_b^{l+1} < r_e^l$ .

Another drawback of Sparse DETR is the insufficient utilization of multi-scale features. In particular, Sparse DETR only flat and concatenate multi-scale feature maps together and does not consider the semantic association between different scales. In addition, the discrepancy in the token selection decisions from different feature maps is also ignored, the semantic association and the discrepancy in the token selection decisions between different scales are ignored, which limits the potential of selecting tokens from the most proper resolution. To fulfill this gap, Focus-DETR constructs the FTS module with top-down score modulations. In order to make full use of the semantic association between multi-scale feature maps, we first use an Multi-Layer Perceptron (MLP) module to predict the foreground score in each feature map. Consid-

ering that high-level feature maps contain richer semantic information than low-level features with higher resolution, we leverage the localization information of high-level semantics as complement information to modulate the feature maps of adjacent low-level semantics. As shown in Fig. 5, unlike the FPN-like feature fusion strategy, our top-down score modulations strategy only transmits foreground scores layer by layer through upsampling. Formally, given the feature map  $f_l$  where  $l \in \{2, 3, 4\}$ , we have

$$S_{l-1} = \text{MLP}_F(f_{l-1}(1 + \text{UP}(\alpha_l * S_l))), \quad (2)$$

where  $S_l$  indicates the foreground score of the  $l$ -th feature map,  $\text{UP}(\cdot)$  is the upsampling function using bilinear interpolation,  $\text{MLP}_F(\cdot)$  is a global score predictor for tokens in all the feature maps,  $\{\alpha_l\}_{l=1}^{L-1}$  is a set of learnable modulation coefficients, and  $L$  indicates the layers of multi-scale feature maps. The localization information of different feature maps is correlated with each other through this type of top-down modulation mechanism.

**Multi-category score predictor.** After selecting tokens with a high probability of falling in the foreground, we then seek an efficient operation to utilize these tokens for better detection performance. Intuitively, we hypothesize that introducing more fine-grained category information would be beneficial in this scenario. Following this motivation, we propose a novel attention mechanism coupled with the foreground token selection to make better use of the token features. As shown in Fig. 3, to avoid meaningless computation of the background token, we employ a stacking strategy that considers both localization information and

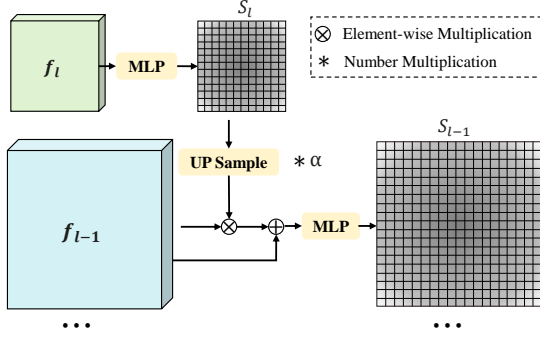

Figure 5: The operation of top-down score modulation. For multi-scale feature maps, we use a shared MLP to calculate  $\{S_1, S_2, \dots\}$ .  $S_l$  is incorporated in the calculation of  $S_{l-1}$  by a dynamic coefficient  $\alpha$  and feature map  $f_{l-1}$ .

category semantic information. Specifically, the product of foreground score and category score calculated by a predictor  $\text{MLP}_C(\cdot)$  will be used as our final criteria  $p_j$  for determining the fine-grained tokens involved in the attention calculation, i.e.,

$$p_j = s_j \times c_j = s_j \times \text{MLP}_C(T_f^j), \quad (3)$$

where  $s_j$  and  $c_j$  represent foreground score and category probabilities of  $T_f^j$  respectively. Unlike the query selection strategy of two-stage Deformable DETR [36] from the encoder’s output, our multi-category probabilities do not include background categories ( $\emptyset$ ).

### 3.3. OESM Pyramid Encoder

**Calculation prototype.** The proposed reliable token scoring mechanism will enable us to perform more fine-grained and discriminatory calculations. After the foreground and fine-grained object tokens are gradually selected based on the scoring mechanism, we first exploit the interaction information of the fine-grained object tokens and corresponding position encoding by an enhanced self-attention. Then, the enhanced object tokens will be scattered back to the original foreground tokens. This way, Focus-DETR can leverage the foreground queries with enhanced semantic information. In addition, because of reliable fine-grained token scoring, Pyramid Encoder effectively boosts the performance with only a negligible increase in calculation cost compared to the unsophisticated query sparse strategy. We utilize Algorithm 1 to illustrate the fine-grained feature selection and enhancement process in detail Pyramid Encoder.

Thus, the proposed module can be viewed as a self-attention layer exploiting the fine-grained object tokens and corresponding position encoding.

**Complexity analysis.** We further analyze the results in

#### Algorithm 1 Encoder equipped with OESM

**Input:** All tokens  $T_a$ , foreground tokens  $T_f$ , position embedding  $PE_f$ , object token number  $k$ , foreground score  $S_f$ , foreground token index  $I_f$

**Output:** all tokens  $T'_a$  and foreground tokens  $T'_f$  after one encoder layer

- 1: category score  $C_f \leftarrow \text{MLP}_C(T_f)$
- 2: maximum of category score  $S_c \leftarrow \max(C_f)$
- 3: object token score  $S_p = S_c \cdot S_f$
- 4:  $Idx_k^{obj} \leftarrow \text{TopK}(S_c, k)$
- 5:  $T_o \leftarrow T_f[Idx_k^{obj}]$ ,  $PE_o \leftarrow PE_f[Idx_k^{obj}]$
- 6:  $q = k = PE_o + T_o$ ,  $v = T_o$
- 7:  $T_o \leftarrow \text{MHSA}(q, k, v)$
- 8:  $T_o \leftarrow \text{Norm}(v + T_o)$
- 9: update  $T_o$  in  $T_f$  according to  $Idx_k^{obj}$
- 10:  $q = T'_f$ ,  $k = T_a + PE_f$ ,  $v = T_a$
- 11:  $T'_f \leftarrow \text{MSDeformAttn}(q, k, v)$
- 12: update  $T'_f$  in  $T_a$  according to  $I_f$

Fig. 2 and our claim that the OESM adds only a negligible calculation cost mathematically. We denote the computational complexity of deformable attention in the encoder and decoder as  $\{G_{DA}^e, G_{DA}^d\}$ , respectively. We calculate  $G_{DA}$  with reference to Deformable DETR [36] as follows:

$$G_{DA} = O(KC + 3MK + C + 5K)N_qC, \quad (4)$$

where  $N_q$  ( $N_q \leq HW = \sum_{i=1}^L h_i w_i$ ) is the number of queries in encoder or decoder,  $K$  is the sampling number in Deformable attention and  $C$  is the embedding dims. For encoder, we set  $N_{qe}$  as  $\gamma HW$ , where  $\gamma$  is the ratio of preserved foreground tokens. For decoder, we set  $N_{qd}$  to be a constant. In addition, the complexity of the self-attention module in decoder is  $O(2N_{qd}C^2 + N_{qd}^2C)$ . For an image whose token number is approximately  $1 \times 10^4$ ,  $\frac{G_{DA}^e}{G_{DA}^d}$  is approximately 7 under the common setting  $\{K = 4, C = 256, N_{qd} = 900, \gamma = 1\}$ . When  $\gamma$  equals 0.3, the calculation cost in the Transformer part will reduce over 60%. This intuitive comparison demonstrates that the encoder is primarily responsible for redundant computing. Then we define the calculation complexity of the OESM as  $G_{OESM}$ :

$$G_{OESM}^d = O(2N_0C^2 + N_0^2C), \quad (5)$$

where  $N_0$  represents the number of fine-grained tokens that obtained by stacking localization information and semantic information. When  $N_0 = 300$ ,  $\frac{G_{OESM}^d}{(G_{DA}^e + G_{DA}^d)}$  is only less than 0.025, which has a negligible impact on the overall model calculation.

### 3.4. Optimization

Like other DETR-like detectors, our model is trained in an end-to-end manner, and the objective function consists

of four parts as follows:

$$\mathcal{L} = \lambda_m \hat{\mathcal{L}}_{match} + \lambda_d \hat{\mathcal{L}}_{dn} + \lambda_f \hat{\mathcal{L}}_f + \lambda_e \hat{\mathcal{L}}_{aux}^{enc}, \quad (6)$$

where  $\hat{\mathcal{L}}_{match}$  is the loss for pair-wise matching based on Hungarian algorithm,  $\hat{\mathcal{L}}_{dn}$  is the loss for denoising following DN-DETR[14],  $\hat{\mathcal{L}}_f$  is the loss for foreground token selector,  $\hat{\mathcal{L}}_{aux}^{enc}$  is the loss for auxiliary optimization through the output of the last encoder layer,  $\lambda_m$ ,  $\lambda_d$ ,  $\lambda_f$ ,  $\lambda_e$  are scaling factors.

**Loss for feature scoring mechanism.** Focus-DETR obtains foreground tokens by the FTS module. Focal Loss [17] is applied to train FTS as follow:

$$\hat{\mathcal{L}}_f = -\alpha_f (1 - p_f)^\gamma \log(p_f), \quad (7)$$

where  $p_f$  represents foreground probability,  $\alpha_f = 0.25$  and  $\gamma = 2$  are empirical hyperparameters.

## 4. Experiments

### 4.1. Experimental Setup

**Dataset:** We conduct experiments on the challenging COCO 2017 [16] detection dataset, which contains 117K training images and 5K validation images. Following the common practice, we report the standard average precision (AP) result on the COCO validation dataset.

**Implementation Details:** The implementation details of Focus-DETR mostly align with the Deformable DETR [36] and the denoising strategy mentioned in DN-DETR [14] and DINO [35] the original model to which it is applied. We adopt ResNet-50 [10], which is pretrained using ImageNet [6] as the backbone and train our model with 8×Nvidia V100 GPUs using the AdamW [12] optimizer. The initial learning rate is set as  $1 \times 10^{-5}$  for the backbone and  $1 \times 10^{-4}$  for the Transformer encoder-decoder framework, with a weight decay of  $1 \times 10^{-4}$ . The learning rate decreases at a later stage by 0.1. The batch size per GPU is set to 2. Model architecture-related hyper-parameters stay the same with DINO [35]. Following DINO, we fix the number of denoising queries and dynamically adjust the number of groups for each image. For the scoring mechanism, the loss weight coefficient of the FTS is set to 1.5. The  $\text{MLP}_C(\cdot)$  shares parameters with the corresponding in the decoder layer and is optimized along with the training of the entire network. In addition, we provide more detailed hyper-parameter settings in Appendix A, including the reserved token ratio in the cascade structure layer by layer and the object scale interval for each layer.

### 4.2. Main Results

Benefiting from the well-designed scoring mechanisms towards the foreground and more informative tokens,

Focus-DETR can focus attention on more fine-grained features, which further improves the performance of the DETR-like model while reducing redundant computations.

Table 1 presents a thorough comparison of the proposed Focus-DETR and other DETR-like detectors [1, 32, 36, 30, 29, 21, 3, 9, 26, 4, 18, 14, 5, 34, 25], as well as Faster R-CNN [24]. When applied to the DINO [35], our Focus-DETR achieves significantly better performance compared with the original DETR baseline (+7.1 AP) and much lower computation cost (18% GFLOPs decrease) for only 36 epochs. For models based on deformable attention [36, 18, 14, 34], Focus-DETR also outperforms Deformable DETR [36] and all variants [18, 14, 4, 34]. We further compare our model with efficient DETR-based detectors [29, 25], our Focus-DETR with keep-ratio of 0.3 outperforms PnP-DETR [29] (+7.9 AP) and Sparse DETR [25] (+4.4 AP). In particular, we also establish a strong baseline by applying the strategy of Sparse DETR to DINO,

In Fig. 6, we plot the AP with GFLOPs to provide a clear picture of the trade-off between accuracy and computation cost. Overall, Our Focus-DETR (DINO version) achieve state-of-the-art performance when compared with prior DETR-like detectors. Compared to original DINO, we lose only 0.5 AP, but the computational cost is reduced by 45% and the inference speed is improved 36%.

To verify the adaptability of Focus-DETR to the stronger backbone ResNet-101 [10] and the effect of the ratio of the preserved foreground on model performance, we perform a series of extensive experiments. As shown in Table 3, compared to other DETR-like models [18, 14, 30, 1, 9, 26, 24], Focus-DETR (DINO version) achieves higher AP with fewer GFLOPs. In addition, when using a Swin Transformer pretrained on ImageNet as our backbone, we can also achieve excellent performance, as shown in Appendix B.1.

### 4.3. Comparison with Sparse DETR

Sparse DETR is state-of-the-art for lightweight DETR-like models but only applies to fixed model that construct decoder queries entirely relying upon encoder selection. As mentioned earlier, sparse DETR’s strategy will cause significant performance degradation when using learnable queries. To verify it, we mainly compare our model with excellent and representative DETR-like models equipped with Sparse DETR strategies, including Deformable DETR, DN-DETR, and DINO. state-of-the-art model DINO [35] and DINO equipped with the strategy of Sparse DETR [25].

In addition to the Sparse two-stage Deformable DETR constructed in the Sparse DETR paper, we apply the Sparse DETR to DN-Deformable DETR and DINO to construct two solid baselines. We retain all the Sparse DETR designs for a fair enough comparison, including the auxiliary encoder loss and related loss weight. We also optimize

| Model                                            | Epochs | AP          | $AP_{50}$ | $AP_{75}$ | $AP_S$ | $AP_M$ | $AP_L$ | Params     | GFLOPs     | FPS         |
|--------------------------------------------------|--------|-------------|-----------|-----------|--------|--------|--------|------------|------------|-------------|
| Faster-RCNN[24]                                  | 108    | 42.0        | 62.4      | 44.2      | 20.5   | 45.8   | 61.1   | 42M        | 180        | 25.3        |
| DETR(DC5)[1]                                     | 500    | 43.3        | 63.1      | 45.9      | 22.5   | 47.3   | 61.1   | 41M        | 187        | 11.2        |
| Efficient-DETR[32]                               | 36     | 44.2        | 62.2      | 48.0      | 28.4   | 47.5   | 56.6   | 32M        | 159        | —           |
| Anchor-DETR-DC5[30]                              | 500    | 44.2        | 64.7      | 47.5      | 24.7   | 48.2   | 60.6   | —          | —          | 19.0        |
| PnP-DETR( $\alpha = 0.33$ )[29]                  | 500    | 42.7        | 62.8      | 45.1      | 22.4   | 46.2   | 60     | —          | —          | 42.5        |
| Conditional-DETR-DC5[21]                         | 108    | 45.1        | 65.4      | 48.5      | 25.3   | 49.0   | 62.2   | 44M        | 195        | 11.5        |
| Conditional-DETR-V2[3]                           | 50     | 44.8        | 65.3      | 48.2      | 25.5   | 48.6   | 62.0   | 46M        | 161        | —           |
| TSP-RCNN-R[26]                                   | 96     | 45.0        | 64.5      | 49.6      | 29.7   | 47.7   | 58.0   | —          | —          | —           |
| Dynamic DETR(5 scales)[4]                        | 50     | 47.2        | 65.9      | 51.1      | 28.6   | 49.3   | 59.1   | 58M        | —          | —           |
| DAB-Deformable-DETR[18]                          | 50     | 46.9        | 66.0      | 50.8      | 30.1   | 50.4   | 62.5   | 44M        | 256        | 14.8        |
| UP-DETR[5]                                       | 300    | 42.8        | 63.0      | 45.3      | 20.8   | 47.1   | 61.7   | —          | —          | —           |
| SAM-DETR[34]                                     | 50     | 45.0        | 65.4      | 47.9      | 26.2   | 49.0   | 63.3   | 58M        | 210        | 24.4        |
| Deformable DETR[36]                              | 50     | 43.8        | 62.6      | 47.7      | 26.4   | 47.1   | 58.0   | 50M        | 173        | 21.2        |
| + Sparse DETR( $\alpha = 0.3$ )[25]              | 50     | 46.0        | 65.9      | 49.7      | 29.1   | 49.1   | 60.6   | 41M        | 121        | 22.4        |
| or + <b>Focus-DETR (Ours)</b> ( $\alpha = 0.3$ ) |        |             |           |           |        |        |        |            |            |             |
| DN-Deformable-DETR[14]                           | 50     | 48.6        | 67.4      | 52.7      | 31.0   | 52.0   | 63.7   | 48M        | 265        | —           |
| + Sparse DETR( $\alpha = 0.3$ )[25]              |        |             |           |           |        |        |        |            |            |             |
| or + <b>Focus-DETR (Ours)</b> ( $\alpha = 0.3$ ) |        |             |           |           |        |        |        |            |            |             |
| DINO[35]                                         | 36     | 50.9        | 69.0      | 55.3      | 34.6   | 54.1   | 64.6   | 47M        | 279        | 13.7        |
| + Sparse DETR( $\alpha = 0.3$ )[25]              | 36     | 48.2        | 65.9      | 52.5      | 30.4   | 51.4   | 63.1   | 47M        | 158        | 18.8        |
| or + <b>Focus-DETR (Ours)</b> ( $\alpha = 0.3$ ) | 36     | <b>50.4</b> | 68.5      | 55.0      | 34.0   | 53.5   | 64.4   | <b>48M</b> | <b>154</b> | <b>18.6</b> |

Table 1: Results for our Focus-DETR and other detection models with the ResNet50 backbone on COCO val2017. Herein,  $\alpha$  indicates the *keep ratio* for methods that prune background tokens. All reported FPS are measured on a NVIDIA V100 GPU.

| Model                     | Epochs | AP   | $AP_{50}$ | $AP_{75}$ | Params | GFLOPs |
|---------------------------|--------|------|-----------|-----------|--------|--------|
| Faster RCNN-FPN [24]      | 108    | 44.0 | 63.9      | 47.8      | 60M    | 246    |
| TSP-RCNN [26]             | 96     | 46.5 | 66.0      | 51.2      | —      | 254    |
| SMCA [9]                  | 50     | 44.4 | 65.2      | 48.0      | 50M    | 218    |
| DETR-DC5 [1]              | 500    | 44.9 | 64.7      | 47.7      | 60M    | 253    |
| Anchor-DETR* [30]         | 50     | 45.1 | 65.7      | 48.8      | 58M    | —      |
| DN DETR [14]              | 50     | 45.2 | 65.5      | 48.3      | 63M    | 174    |
| DN DETR-DC5 [14]          | 50     | 47.3 | 67.5      | 50.8      | 63M    | 282    |
| DN-Deformable DETR [14]   | 12     | 44.1 | 62.8      | 47.9      | 67M    | 275    |
| Conditional DETR-DC5 [21] | 108    | 45.9 | 66.8      | 49.5      | 63M    | 262    |
| DAB DETR-DC5 [18]         | 50     | 46.6 | 67.0      | 50.2      | 63M    | 296    |
| <b>Focus-DETR (Ours)</b>  | 36     | 51.4 | 70.0      | 55.7      | 67M    | 221    |

Table 3: Comparison of the proposed Focus-DETR and other models with ResNet101 backbone. Our Focus-DETR preserve 30% tokens after the backbone. The models with superscript \* use 3 pattern embeddings as in Anchor DETR [30].

these baselines by adjusting hyperparameters to achieve the best performance. As shown in Table 2, when applying Sparse DETR to Deformable DETR without two-stage, DN-Deformable-DETR and DINO, the AP decreases 1.9, 1.2 and 2.0, and the correlations between DAM and retained foreground tokens are far lower than original Sparse DETR.

our method achieves 2.2 higher AP with similar latency. Compared to Sparse DETR, Focus-DETR achieves x.x, 2.2 and x.x higher AP with similar la-

tency in Deformable DETR(two-stage off), DINO and DN-Deformable DETR. Intriguingly, Focus-DETR even obtain comparable performance with the unpruned DINO model with significantly lower computation cost (18.6 FPS vs. 13.7 FPS).

#### 4.4. Ablation Studies

We conduct ablation studies to validate the effectiveness of our proposed components. Experiments are performed

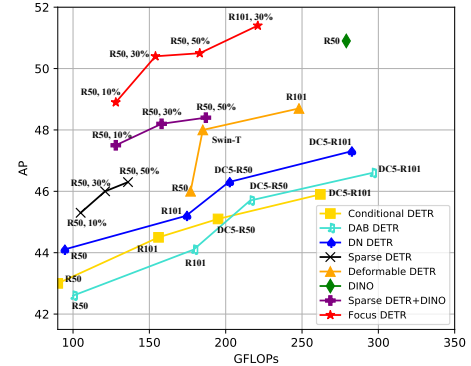

Figure 6: Performance of recent object detectors in terms of average precision (AP) and GFLOPs. The GFLOPs is measured using 100 validation images.



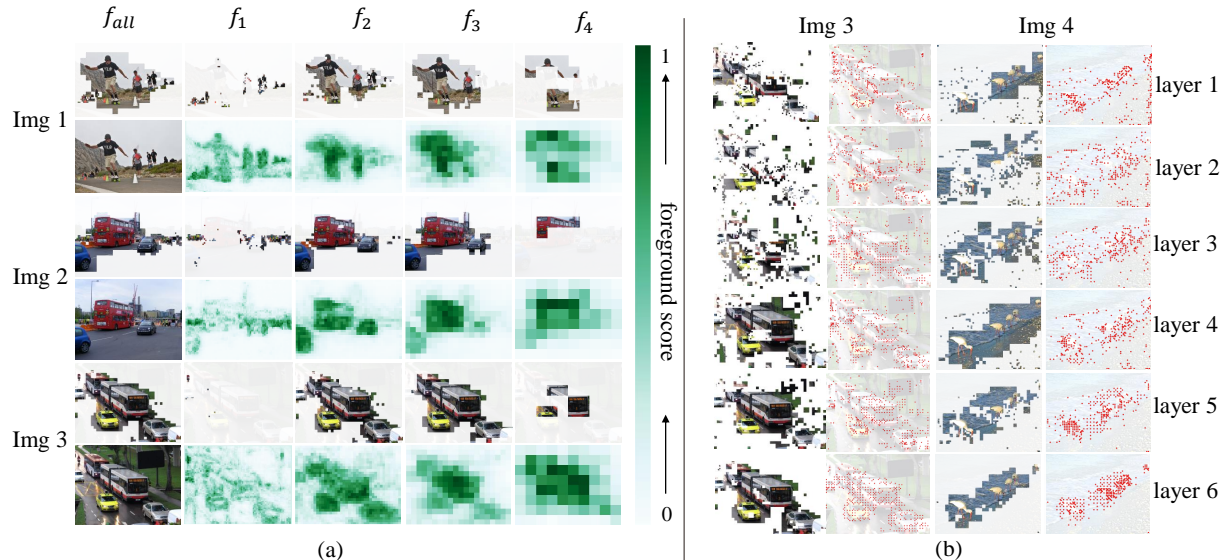

Figure 7: Visualization results of preserved foreground tokens distribution at multi-scale feature maps as shown (a) and  $k$  object tokens evolution at different encoder layers as shown (b). {Img1, Img2, Img3, Img4} represent four test images,  $\{f_1, f_2, f_3, f_4\}$  represent foreground tokens at four feature maps, {layer 1, layer 2 ...} represent different encoder layers.

Table 2: *Corr*: the correlation of DAM and retained foreground(5k validation set). “**priori**”: position and content query (encoder selection); “**learnable**”: position and content query (initialization); “**mixed**”: position query (encoder selection), content query (initialization).

| Model                                                    | AP | Corr                                       | GFLOPs | FPS |
|----------------------------------------------------------|----|--------------------------------------------|--------|-----|
| Deformable DETR ( <b>priori</b> )<br>+ Sparse DETR       | 50 | $0.5784 \pm 0.0682$<br>$0.5784 \pm 0.0682$ |        |     |
| Deformable DETR ( <b>learnable</b> )<br>+ Sparse DETR    |    | $0.5784 \pm 0.0682$<br>$0.5784 \pm 0.0682$ |        |     |
| DN-Deformable-DETR ( <b>learnable</b> )<br>+ Sparse DETR |    | $0.5784 \pm 0.0682$<br>$0.5784 \pm 0.0682$ |        |     |
| DINO ( <b>mixed</b> )<br>+ Sparse DETR                   |    | $0.5784 \pm 0.0682$<br>$0.5784 \pm 0.0682$ |        |     |

| FTS       |             | score<br>modulations | cascade | OESM | AP          | $AP_{50}$   | $AP_{75}$   | FPS  |
|-----------|-------------|----------------------|---------|------|-------------|-------------|-------------|------|
| predictor | supervision |                      |         |      |             |             |             |      |
| ✓         |             |                      |         |      | 47.8        | 65.2        | 52.1        | 19.4 |
| ✓         | ✓           |                      |         |      | 48.6        | 66.2        | 53.2        | 19.3 |
| ✓         | ✓           | ✓                    |         |      | 49.2        | 66.4        | 53.7        | 19.2 |
| ✓         | ✓           | ✓                    | ✓       |      | 49.7        | 66.9        | 54.1        | 19.2 |
| ✓         | ✓           | ✓                    | ✓       | ✓    | <b>50.4</b> | <b>68.5</b> | <b>55.0</b> | 18.6 |

Table 4: Ablation studies on the proposed FTS and OESM. FTS is the foreground token selector. OESM represents the Object Enhanced Self-attention Module. Supervision indicates the label assignment from the ground truth bounding boxes.

with ResNet-50 as the backbone using 36 epochs.

**Effect of foreground token selection strategy.** Firstly, simply obtaining the token score using a foreground score predictor without supervision achieves only 47.8 AP and is lower than that (48.2 AP) of DINO pruned by Sparse

| Top-down | Bottom-up | AP                          | $AP_{50}$                   | $AP_{75}$                   |
|----------|-----------|-----------------------------|-----------------------------|-----------------------------|
| ✓        |           | 49.7<br><b>50.4</b><br>50.2 | 66.9<br><b>68.5</b><br>68.4 | 54.0<br><b>55.0</b><br>54.6 |

Table 5: Ablation studies on how to utilize the association between scores of multi-scale feature maps. We try top-down and bottom-up scoring modulations.

DETR. As shown in the second row of Table 4, by adding supervision with our improved label assignment strategy, Focus-DETR yields a significant improvement of +0.8 AP. In addition, top-down score modulations optimize the performance of FTS by enhancing the scoring interaction between multi-scale feature maps. As shown in the third row of Table 4, Focus-DETR equipped with the top-down score modulation achieves +0.6 AP. As the visualization shown in Fig. 7 (a), we can observe that our method precisely select the foreground tokens. Moreover, feature maps in different levels tend to focus on objects with different scales. Furthermore, we find that there is an overlap between the object scales predicted by adjacent feature maps due to our scale overlap setting. We provide more detailed overlap setting details in the Appendix A.2.

**Effect of cascade token selection.** When we keep a fixed number of tokens in the encoder, the high error rate of pre-selection and the accumulation of errors layer by layer is detrimental to the detection performance. To increase the fault tolerance performance of the scoring mechanism, we design the cascade structure for the encoder to reduce the



| Model                                         | $\alpha$ | AP   | AP <sub>50</sub> | AP <sub>75</sub> | AP <sub>S</sub> | AP <sub>M</sub> | AP <sub>L</sub> | GFLOPs | FPS |
|-----------------------------------------------|----------|------|------------------|------------------|-----------------|-----------------|-----------------|--------|-----|
| Sparse DETR [25]<br>(epoch=50)                | 0.1      | 45.3 | 65.8             | 49.3             | 28.4            | 48.3            | 60.1            | 105    |     |
|                                               | 0.2      | 45.6 | 65.8             | 49.6             | 28.5            | 48.6            | 60.4            | 113    |     |
|                                               | 0.3      | 46.0 | 65.9             | 49.7             | 29.1            | 49.1            | 60.6            | 121    |     |
|                                               | 0.4      | 46.2 | 66.0             | 50.3             | 28.7            | 49.0            | 61.4            | 128    |     |
|                                               | 0.5      | 46.3 | 66.0             | 50.1             | 29.0            | 49.5            | 60.8            | 136    |     |
| DINO [35]<br>+ Sparse DETR [25]<br>(epoch=36) | 0.1      | 47.5 | 64.9             | 51.7             | 29.1            | 50.7            | 62.7            | 128    |     |
|                                               | 0.2      | 47.9 | 65.6             | 52.1             | 30.0            | 51.1            | 62.9            | 143    |     |
|                                               | 0.3      | 48.2 | 66.0             | 52.5             | 30.5            | 51.4            | 63.1            | 158    |     |
|                                               | 0.4      | 48.4 | 66.2             | 52.5             | 30.5            | 51.8            | 63.2            | 172    |     |
|                                               | 0.5      | 48.4 | 66.1             | 52.6             | 30.6            | 51.8            | 63.4            | 187    |     |
| <b>Focus-DETR</b><br>(epoch=36)               | 0.1      | 48.9 | 67.0             | 53.2             | 32.6            | 52.6            | 64.1            | 128    |     |
|                                               | 0.2      | 49.8 | 67.9             | 54.1             | 32.3            | 52.9            | 64.0            | 141    |     |
|                                               | 0.3      | 50.4 | 68.4             | 55.1             | 33.9            | 53.5            | 64.4            | 154    |     |
|                                               | 0.4      | 50.4 | 68.4             | 55.2             | 34.0            | 53.7            | 64.1            | 169    |     |
|                                               | 0.5      | 50.5 | 68.6             | 54.9             | 34.4            | 53.8            | 64.0            | 183    |     |

Table 6: Experiment results in detection performance and model complexity when changing the ratio of foreground tokens retained by Focus-DETR, Sparse DETR, and DINO+Sparse DETR.

number of foreground tokens layer by layer (Section 3.2). As shown in Fig. 7 (b), we can see the fine-grained tokens focusing process in the encoder as the selecting range decreases, which enhances the model’s fault tolerance and further improves the model’s performance. As illustrated in the fourth row of Table 4, Focus-DETR equipped with cascade structure achieves +0.5 AP.

**Effect of Object Enhanced Self-attention Module.** Compared with the solutions of PnP-DETR [29] and Sparse DETR [25] that abandon the background token, one of our core contributions is to further enhance fine-grained tokens with negligible computational cost. We perform experiments to analyze the effects of the OESM on the semantic enhancement of fine-grained object tokens. As shown in the fifth row of Table 4, OESM brings 0.8 AP improvement. These results demonstrate that enhancing fine-grained tokens is beneficial to boost detection performance and the effectiveness of our stacked position and semantic information for fine-grained feature selection, as shown in Fig. 1.

**Effect of top-down score modulation.** We further analysis the effect of the multi-scale scoring guidance mechanisms in our method. As shown in Table 5, we can observe that utilizing multi-scale information for score prediction brings consistent improvement (+0.5 or +0.7 AP). We also conduct ablation experiments for different score modulation methods. The proposed top-down score guidance strategy (Section 3.2) achieves 0.2 higher AP than bottom-down strategy, which justifies our motivation that using high-level scores to modulating low-level foreground probabilities is beneficial for the final performance.

**Effect of pruning ratio.** As shown in Table 6 and Fig. 8, we analyze the detection performance and model complexity when changing the ratio of foreground tokens retained

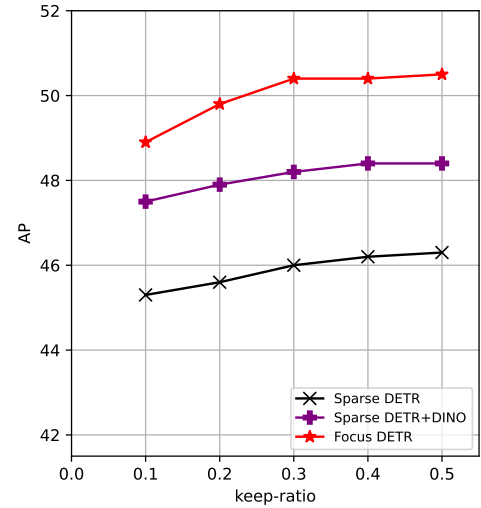

Figure 8: Performance of different object detectors in terms of average precision (AP) and ratio of foreground tokens.

by different methods. Focus-DETR achieves optimal performance when keeping the same ratio. Specifically, Focus-DETR achieves +2.7 AP than Sparse DETR and +1.4AP than DINO equipped with Sparse DETR’s strategies with similar computation cost at 128 GFLOPs.

#### 4.5. Limitation and Future Directions

Although Focus-DETR has designed a delicate token scoring mechanism and fine-grained feature enhancement methods, more hierarchical semantic grading strategies, such as object boundaries or centers, are still worth exploring. In addition, our future work will be constructing a unified feature semantic scoring mechanism and fine-grained feature enhancement algorithm throughout the Transformer.

## 5. Conclusion

This paper proposes Focus-DETR to focus on more informative tokens for a better trade-off between computation efficiency and model accuracy. The core component of Focus-DETR is a multi-level discrimination strategy for feature semantics that utilizes a scoring mechanism considering both position and semantic information. Focus-DETR achieves a better trade-off between computation efficiency and model accuracy by precisely selecting foreground and fine-grained tokens for enhancement. Experimental results show that Focus-DETR has become the SOTA method in token pruning for DETR-like models. Our work is instructive for the design of transformer-based detectors.

## References

- [1] Nicolas Carion, Francisco Massa, Gabriel Synnaeve, Nicolas Usunier, Alexander Kirillov, and Sergey Zagoruyko. End-

- to-end object detection with transformers. In European Conference of Computer Vision, 2020. 1, 2, 6, 7
- [2] Qiang Chen, Xiaokang Chen, Gang Zeng, and Jingdong Wang. Group DETR: fast training convergence with decoupled one-to-many label assignment. CoRR, abs/2207.13085, 2022. 1, 2
- [3] Xiaokang Chen, Fangyun Wei, Gang Zeng, and Jingdong Wang. Conditional DETR V2: efficient detection transformer with box queries. CoRR, abs/2207.08914, 2022. 2, 6, 7
- [4] Xiyang Dai, Yinpeng Chen, Jianwei Yang, Pengchuan Zhang, Lu Yuan, and Lei Zhang. Dynamic detr: End-to-end object detection with dynamic attention. In International Conference on Computer Vision, pages 2968–2977, 2021. 2, 6, 7
- [5] Zhigang Dai, Bolun Cai, Yugeng Lin, and Junying Chen. Up-detr: Unsupervised pre-training for object detection with transformers. In Computer Vision and Pattern Recognition, pages 1601–1610, 2021. 2, 6, 7
- [6] Jia Deng, Wei Dong, Richard Socher, Li-Jia Li, Kai Li, and Li Fei-Fei. Imagenet: A large-scale hierarchical image database. In Computer Vision and Pattern Recognition, pages 248–255, 2009. 6
- [7] Alexey Dosovitskiy, Lucas Beyer, Alexander Kolesnikov, Dirk Weissenborn, Xiaohua Zhai, Thomas Unterthiner, Mostafa Dehghani, Matthias Minderer, Georg Heigold, Sylvain Gelly, Jakob Uszkoreit, and Neil Houlsby. An image is worth 16x16 words: Transformers for image recognition at scale. In AAAI Conference on Artificial Intelligence. OpenReview.net, 2021. 2
- [8] Yuxin Fang, Bencheng Liao, Xinggang Wang, Jiemin Fang, Jiyang Qi, Rui Wu, Jianwei Niu, and Wenyu Liu. You only look at one sequence: Rethinking transformer in vision through object detection. arXiv preprint arXiv:2106.00666, 2021. 2
- [9] Peng Gao, Minghang Zheng, Xiaogang Wang, Jifeng Dai, and Hongsheng Li. Fast convergence of detr with spatially modulated co-attention. In International Conference on Computer Vision, pages 3601–3610, 2021. 6, 7
- [10] Kaiming He, Xiangyu Zhang, Shaoqing Ren, and Jian Sun. Deep residual learning for image recognition. In Computer Vision and Pattern Recognition, pages 770–778, 2016. 3, 6
- [11] Sehoon Kim, Sheng Shen, David Thorsley, Amir Gholami, Woosuk Kwon, Joseph Hassoun, and Kurt Keutzer. Learned token pruning for transformers. In Aidong Zhang and Huzefa Rangwala, editors, Knowledge Discovery and Data Mining, pages 784–794. ACM, 2022. 3
- [12] Diederik P. Kingma and Jimmy Ba. Adam: A method for stochastic optimization. In Yoshua Bengio and Yann LeCun, editors, International Conference on Learning Representations, 2015. 6
- [13] Zhenglun Kong, Peiyan Dong, Xiaolong Ma, Xin Meng, Wei Niu, Mengshu Sun, Bin Ren, Minghai Qin, Hao Tang, and Yanzhi Wang. Spvit: Enabling faster vision transformers via soft token pruning. ArXiv, abs/2112.13890, 2021. 3
- [14] Feng Li, Hao Zhang, Shilong Liu, Jian Guo, Lionel M Ni, and Lei Zhang. Dn-detr: Accelerate detr training by introducing query denoising. In Computer Vision and Pattern Recognition, 2022. 1, 2, 6, 7
- [15] Yanghao Li, Hanzi Mao, Ross Girshick, and Kaiming He. Exploring plain vision transformer backbones for object detection. arXiv preprint arXiv:2203.16527, 2022. 2
- [16] Tsung-Yi Lin, Michael Maire, Serge J. Belongie, James Hays, Pietro Perona, Deva Ramanan, Piotr Dollár, and C. Lawrence Zitnick. Microsoft COCO: common objects in context. In David J. Fleet, Tomás Pajdla, Bernt Schiele, and Tinne Tuytelaars, editors, European Conference of Computer Vision, volume 8693 of Lecture Notes in Computer Science, pages 740–755. Springer, 2014. 6
- [17] Tsung-Yi Lin, Priya Goyal, Ross Girshick, Kaiming He, and Piotr Dollár. Focal loss for dense object detection. IEEE Transactions on Pattern Analysis and Machine Intelligence, 42(2):318–327, 2020. 3, 6
- [18] Shilong Liu, Feng Li, Hao Zhang, Xiao Yang, Xianbiao Qi, Hang Su, Jun Zhu, and Lei Zhang. DAB-DETR: Dynamic anchor boxes are better queries for DETR. In International Conference on Learning Representations, 2022. 1, 2, 6, 7
- [19] Xiangcheng Liu, Tianyi Wu, and Guodong Guo. Adaptive sparse vit: Towards learnable adaptive token pruning by fully exploiting self-attention. CoRR, abs/2209.13802, 2022. 3
- [20] Ze Liu, Yutong Lin, Yue Cao, Han Hu, Yixuan Wei, Zheng Zhang, Stephen Lin, and Baining Guo. Swin transformer: Hierarchical vision transformer using shifted windows. In International Conference on Computer Vision (ICCV), 2021. 3
- [21] Depu Meng, Xiaokang Chen, ZeJia Fan, Gang Zeng, Houqiang Li, Yuhui Yuan, Lei Sun, and Jingdong Wang. Conditional detr for fast training convergence. In International Conference on Computer Vision (ICCV), 2021. 1, 2, 6, 7
- [22] Bowen Pan, Yifan Jiang, Rameswar Panda, Zhangyang Wang, Rogério Feris, and Aude Oliva. Ia-red<sup>2</sup>: Interpretability-aware redundancy reduction for vision transformers. CoRR, abs/2106.12620, 2021. 2
- [23] Yongming Rao, Wenliang Zhao, Benlin Liu, Jiwen Lu, Jie Zhou, and Cho-Jui Hsieh. Dynamicvit: Efficient vision transformers with dynamic token sparsification. In Advances in Neural Information Processing Systems, 2021. 3
- [24] Shaoqing Ren, Kaiming He, Ross Girshick, and Jian Sun. Faster r-cnn: Towards real-time object detection with region proposal networks. In C. Cortes, N. Lawrence, D. Lee, M. Sugiyama, and R. Garnett, editors, Advances in Neural Information Processing Systems, volume 28. Curran Associates, Inc., 2015. 6, 7
- [25] Byungseok Roh, JaeWoong Shin, Wuhyun Shin, and Sehoon Kim. Sparse DETR: Efficient end-to-end object detection with learnable sparsity. In International Conference on Learning Representations, 2022. 1, 2, 3, 6, 7, 9
- [26] Zhiqing Sun, Shengcao Cao, Yiming Yang, and Kris Kitani. Rethinking transformer-based set prediction for object detection. In International Conference on Computer Vision, pages 3591–3600, 2021. 6, 7
- [27] Yehui Tang, Kai Han, Yunhe Wang, Chang Xu, Jianyuan Guo, Chao Xu, and Dacheng Tao. Patch slimming for ef-

- efficient vision transformers. In Computer Vision and Pattern Recognition (CVPR), pages 12155–12164, 2022. 3
- [28] Zhi Tian, Chunhua Shen, Hao Chen, and Tong He. Fcos: Fully convolutional one-stage object detection. In International Conference on Computer Vision (ICCV), pages 9626–9635, 2019. 3
- [29] Tao Wang, Li Yuan, Yunpeng Chen, Jiashi Feng, and Shuicheng Yan. Pnp-detr: Towards efficient visual analysis with transformers. In International Conference on Computer Vision, 2021. 1, 2, 3, 6, 7, 9
- [30] Yingming Wang, Xiangyu Zhang, Tong Yang, and Jian Sun. Anchor detr: Query design for transformer-based detector. In AAAI Conference on Artificial Intelligence, 2022. 1, 6, 7
- [31] Yifan Xu, Zhijie Zhang, Mengdan Zhang, Kekai Sheng, Ke Li, Weiming Dong, Liqing Zhang, Changsheng Xu, and Xing Sun. Evo-vit: Slow-fast token evolution for dynamic vision transformer. In AAAI Conference on Artificial Intelligence, volume 36, pages 2964–2972, 2022. 3
- [32] Zhuyu Yao, Jiangbo Ai, Boxun Li, and Chi Zhang. Efficient DETR: improving end-to-end object detector with dense prior. CoRR, abs/2104.01318, 2021. 1, 3, 6, 7
- [33] Hongxu Yin, Arash Vahdat, Jose M. Alvarez, Arun Mallya, Jan Kautz, and Pavlo Molchanov. A-vit: Adaptive tokens for efficient vision transformer. In Computer Vision and Pattern Recognition (CVPR), pages 10799–10808, 2022. 3
- [34] Gongjie Zhang, Zhipeng Luo, Yingchen Yu, Kaiwen Cui, and Shijian Lu. Accelerating detr convergence via semantic-aligned matching. In Computer Vision and Pattern Recognition (CVPR), pages 939–948, 2022. 2, 6, 7
- [35] Hao Zhang, Feng Li, Shilong Liu, Lei Zhang, Hang Su, Jun Zhu, Lionel M. Ni, and Heung-Yeung Shum. Dino: Detr with improved denoising anchor boxes for end-to-end object detection, 2022. 1, 2, 6, 7, 9
- [36] Xizhou Zhu, Weijie Su, Lewei Lu, Bin Li, Xiaogang Wang, and Jifeng Dai. Deformable detr: Deformable transformers for end-to-end object detection. In International Conference on Learning Representations, 2021. 1, 2, 5, 6, 7

1134  
1135  
1136  
1137  
1138  
1139  
1140  
1141  
1142  
1143  
1144  
1145  
1146  
1147  
1148  
1149  
1150  
1151  
1152  
1153  
1154  
1155  
1156  
1157  
1158  
1159  
1160  
1161  
1162  
1163  
1164  
1165  
1166  
1167  
1168  
1169  
1170  
1171  
1172  
1173  
1174  
1175  
1176  
1177  
1178  
1179  
1180  
1181  
1182  
1183  
1184  
1185  
1186  
1187
